# Supplementary material for: From unicellular fatgraphs to trees
Source: arXiv:1806.03319 source file (2018-06-08)
Supplement: Supplementary file 1 [file SupplementaryMaterial.pdf]

# Supplementary Material

Thomas J. X. Li, Christian M. Reidys*

*Biocomplexity Institute of Virginia Tech*
*1015 Life Sciences Circle, Blacksburg, VA 24061, USA*

*Department of Mathematics of Virginia Tech*
*225 Stanger Street, Blacksburg, VA 24061, USA*

## 1. Proofs of Proposition 2 and Proposition 3

To define the fatgraph $\mathbb{G}^C$ induced by a component $C$, we first study the trace $I_C$.

**Proposition 1.** *Let $C$ be a component with trace, $I_C = \dot\cup_i^l [a_i, c_i]_\gamma$ and let $r$ be a ribbon not in $C$. Then either $\{r^L, \gamma(r^L), \gamma^{-1}(r^R), r^R\} \subset [1, a_1]_\gamma \dot\cup [c_l, 2n+1]_\gamma$ or $\{r^L, \gamma(r^L), \gamma^{-1}(r^R), r^R\} \subset [c_k, a_{k+1}]_\gamma$ for some $1 \le k \le l$ (where $a_{l+1} = a_1$ and $[c_l, a_{l+1}]_\gamma = [1, a_1]_\gamma \dot\cup [c_l, 2n+1]_\gamma$).*

*Proof.* For any ribbon $r_1$ that is non-crossing with $r$, we have four cases: $r^L <_\gamma r_1^L <_\gamma r_1^R <_\gamma r^R$, $r_1^L <_\gamma r^L <_\gamma r^R <_\gamma r_1^R$, $r_1^L <_\gamma r_1^R \le_\gamma r^L <_\gamma r^R$ or $r^L <_\gamma r^R \le_\gamma r_1^L <_\gamma r_1^R$. I.e. all sectors $\{r_1^L, \gamma(r_1^L), \gamma^{-1}(r_1^R), r_1^R\}$ must be contained in either $(r^L, r^R)_\gamma$ or $[1, r^L]_\gamma \dot\cup [r^R, 2n+1]_\gamma$. Since $r \notin C$, it follows from the definition of a component that all ribbons of $C$ are not crossing with $r$ and thus all their sectors must be contained in either $(r^L, r^R)_\gamma$ or $[1, r^L]_\gamma \dot\cup [r^R, 2n+1]_\gamma$. Therefore, we have either $I_C \subset (r^L, r^R)_\gamma$ or $I_C \subset [1, r^L]_\gamma \dot\cup [r^R, 2n+1]_\gamma$, which implies that either $\{r^L, \gamma(r^L), \gamma^{-1}(r^R), r^R\} \subset [1, a_1]_\gamma \dot\cup [c_l, 2n+1]_\gamma$ or $\{r^L, \gamma(r^L), \gamma^{-1}(r^R), r^R\} \subset [c_k, a_{k+1}]_\gamma$ for some $1 \le k \le l-1$. □

**Proposition 2.** *Let $C$ be a component with $I_C = \dot\cup_i^l [a_i, c_i]_\gamma$. Then*
(1) *$c_k, a_{k+1}$ are located at the same vertex and have the same orientation for*

*Corresponding author.
*Email addresses:* thomasli@vt.edu (Thomas J. X. Li), duck@santafe.edu (Christian M. Reidys)

$1 \le k \le l$,
(2) *let*

$$F(c_k, a_{k+1}) = \begin{cases} \{s\colon\ c_k <_\sigma s <_\sigma a_{k+1}\} & \textit{if } \omega(c_k) = \omega(a_{k+1}) = +1 \\ \{s\colon\ a_{k+1} <_\sigma s <_\sigma c_k\} & \textit{if } \omega(c_k) = \omega(a_{k+1}) = -1, \end{cases}$$

*be the* fan *of* $c_k$ *and* $a_{k+1}$. *Then* $F(c_k, a_{k+1}) \cap I_C = \varnothing$.

*Proof.* To prove (1), suppose $c_k$ is located at vertex $v$ and without loss of generality we may assume that $c_k$ has counterclockwise orientation. The proof for $c_k$ being clockwise oriented is completely analogous. Set $q = \min\{h \ge 1\colon\ \sigma^h(c_k) \in I_C\}$. By definition we have $c_k \in I_C$ and such a $q$ always exists.

Let $r_1, \dots, r_q, r_{q+1}$ be the sequence of ribbons incident to $v$, labeled clockwise starting from $c_k$ around $v$. By construction, $r_h$ is associated to the sectors $\sigma^{h-1}(c_k)$ and $\sigma^h(c_k)$, see Fig. 1.

*Claim.* $r_1, \dots, r_q$ are not $C$-ribbons and furthermore $\sigma(c_k), \dots, \sigma^q(c_k) \in [c_k, a_{k+1}]_\gamma$.

To prove the claim we observe that $r_1$ is associated with three sectors $c_k$, $\sigma(c_k)$, and $c_k + 1$, where sector $c_k + 1$ is, by definition, not contained in $I_C$. This implies that $r_1$ is not a $C$-ribbon. By Proposition 1, we have $\sigma(c_k) \in [c_k, a_{k+1}]_\gamma$.

We proceed by induction, using the above as induction basis: suppose the claim holds for $r_{j-1}$ and $\sigma^{j-1}(c_k)$. By definition of $q$, we have $\sigma^{j-1}(c_k), \sigma^j(c_k) \notin I_C$ and $r_j$ is associated with the sectors $\sigma^{j-1}(c_k), \sigma^j(c_k)$. As a result, $r_j$ is not a $C$-ribbon. By the induction hypothesis we have $\sigma^{j-1}(c_k) \in [c_k, a_{k+1}]_\gamma$ and Proposition 1, applied to $r_j$, implies $\sigma^j(c_k) \in [c_k, a_{k+1}]_\gamma$ and the claim holds.

According to the claim we have $\sigma^q(c_k) \in [c_k, a_{k+1}]_\gamma$ and by construction $\sigma^q(c_k) \in I_C$, i.e., $\sigma^q(c_k) \in [c_k, a_{k+1}]_\gamma \cap I_C$. As a result we are left with the alternative $\sigma^q(c_k) = c_k$ or $\sigma^q(c_k) = a_{k+1}$. In case of $\sigma^q(c_k) = c_k$, $C$ contains exclusively $c_k$ at $v$. There are two ribbons that contain the sector $c_k$, one associated to $c_k, \sigma^{-1}(c_k)$ and the other to $c_k, \sigma(c_k)$. Since $\sigma^q(c_k) = c_k$, neither $\sigma^{-1}(c_k)$ nor $\sigma(c_k)$ can be contained in $C$, which is a contradiction. Therefore $\sigma^q(c_k) = a_{k+1}$, i.e., $c_k$ and $a_{k+1}$ are located at the same vertex.

Since $\sigma^q(c_k) \in I_C$ is associated with two ribbons $r_q, r_{q+1}$ and $r_q \notin C$, we derive $r_{q+1} \in C$. This implies that $r_{q+1}$ has to contain the sectors $a_{k+1}, a_{k+1} + 1$ and we can conclude from this that $a_{k+1}$ has counterclockwise orientation, see Fig. 1 and assertion (1) is proved.

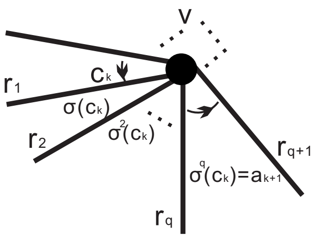


**Fig.** 1: Sectors in a component.

To prove (2), we observe that, by construction,

$$F(c_k, a_{k+1}) = \{\sigma(c_k), \ldots, \sigma^{q-1}(c_k)\} \subset (c_k, a_{k+1})_\gamma$$

and $F(c_k, a_{k+1}) \cap I_C = \varnothing$. This holds for any pair $\{c_k, a_{k+1}\}$, whence (2). □

Given a permutation $\alpha$ on $[2n+1]$ and $N \subset [2n+1]$, the *restriction* $\alpha|_N$ of $\alpha$ is the permutation on $N$ having the cycle representation obtained from that of $\alpha$ by removing all elements which are not in $N$, i.e., for any $i \in N$, $\alpha|_N(i) = \alpha^m(i)$, where $m = \min\{l \geq 1\colon\ \alpha^l(i) \in N\}$.

Now we are in position to define the unicellular fatgraph $\mathbb{G}^C$ *induced* by a component $C$, see Fig. 2. Suppose that $C$ has trace $I_C = \dot{\cup}_i^l [a_i, c_i]_\gamma$. Then $\mathbb{G}^C = (I', \sigma', \gamma', \omega')$, where the set $I'$ consists of the sectors of $I_C$ obtained by identifying sectors $c_k$ and $a_{k+1}$ as $h_k$, for $1 \leq k \leq l-1$, the permutations $\sigma'$ and $\gamma'$ are obtained from $\sigma|_{I_C}$ and $\gamma|_{I_C}$ by identifying sectors $c_k$ and $a_{k+1}$ as the new sector $h_k$, respectively and $\omega'$ is the restriction of $\omega$ satisfying $\omega'(h_k) = \omega(c_k) = \omega(a_{k+1})$.

By Proposition 2, $c_k$ and $a_{k+1}$ are located at the same vertex and $F(c_k, a_{k+1}) \cap I_C = \varnothing$, implying that $\sigma|_{I_C}(c_k) = a_{k+1}$ (we shall assume here, without loss of generality, that $c_k$ and $a_{k+1}$ are counterclockwise oriented) and $\sigma'(\sigma^{-1}|_{I_C}(c_k)) = h_k, \sigma'(h_k) = \sigma|_{I_C}(a_{k+1})$. In view of these facts $\sigma'$ is well-defined, see Fig. 2. Clearly, $\gamma'$ and $\omega'$ are well-defined.

*Proof of Proposition 2.* We shall show that $\mathbb{G}^C$ is unicellular and irreducible. By construction, $\mathbb{G}^C$ has the boundary component $\gamma' = (a_1, \ldots, c_1 - 1, h_1, a_2 + 1, \ldots, c_2 - 1, h_2, a_3 + 1, \ldots, c_l - 1, h_l, a_{l+1} + 1, \ldots, c_l)$. Since $\gamma'$ has only one cycle, $\mathbb{G}^C$ is unicellular.

**Claim:** any two $\mathbb{G}$-crossing ribbons $r_1$ and $r_2$ of $C$ are $\mathbb{G}^C$-crossing, when considered in $\mathbb{G}^C$.

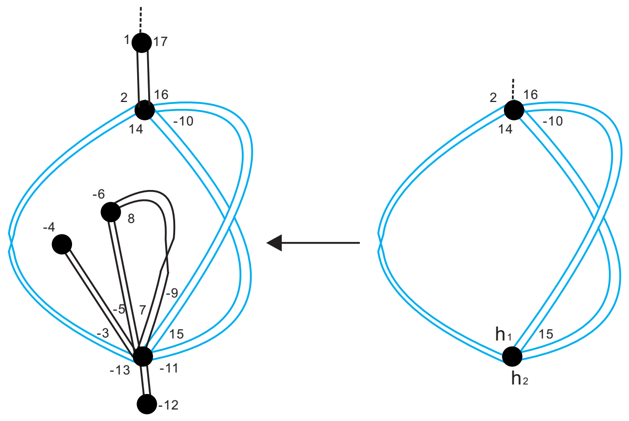


**Fig.** 2: The unicellular fatgraph $\mathbb{G}^C$ induced by a component $C$.

By definition, $r_1^L <_\gamma r_2^L <_\gamma r_1^R <_\gamma r_2^R$ or $r_2^L <_\gamma r_1^L <_\gamma r_2^R <_\gamma r_1^R$. Note that $\gamma'$ is obtained from $I_C$ by identifying $c_k$ and $a_{k+1}$, where $c_k <_\gamma a_{k+1}$, $c_k$ is the terminus and $a_{k+1}$ is the origin of a $C$-ribbon. Accordingly, the order of the sectors of $r_1, r_2$ is the same in $\gamma$ and $\gamma'$ and $r_1, r_2$ are $\mathbb{G}^C$-crossing, if they are crossing in $\mathbb{G}$.

Any two $C$-ribbons $r_1$ and $r_2$ are $\mathbb{G}$-associated. That is, there exists a sequence of $C$-ribbons $(r_1 = w_1, w_2, \ldots, w_{k-1}, w_k = r_2)$ such that $w_i$ and $w_{i+1}$ are $\mathbb{G}$-crossing. By the claim, $w_i, w_{i+1}$ are $\mathbb{G}^C$-crossing, which implies that $r_1$ and $r_2$ are $\mathbb{G}^C$-associated, whence $\mathbb{G}^C$ is irreducible. □

*Proof of Proposition 3.* Let $C_1$ and $C_2$ be two components. Assume that $I_{C_1} = \cup_i^{l_1}[a_i^{(1)}, c_i^{(1)}]_\gamma$ and $I_{C_2} = \cup_j^{l_2}[a_j^{(2)}, c_j^{(2)}]_\gamma$. We shall show that $I_{C_2} \subset [c_k^{(1)}, a_{k+1}^{(1)}]_\gamma$ for some $k$ with $1 \leq k \leq l_1$.

Given a $C_2$-ribbon $r$, Proposition 1 shows that the set of $r$-sectors is contained in $[c_{k(r)}^{(1)}, a_{k(r)+1}^{(1)}]_\gamma$ for some $k(r)$ with $1 \leq k(r) \leq l_1$. It remains to show that $k(r)$ does not depend on $r$. Let $r_1$ and $r_2$ be two crossing $C_2$-ribbons. Since $r_1^L <_\gamma r_2^L <_\gamma r_1^R <_\gamma r_2^R$, their sets of sectors are contained in the same gap, i.e., $k(r_1) = k(r_2)$. Note that any two $C_2$-ribbons are associated. Thus the sets of sectors of any two $C_2$-ribbons are contained in the same gap, completing the proof. □

## 2. Proof of Lemma 2

**Proposition 3.** *Let $e_1$ denote the ribbon containing $i, i+1$ and $e_2$ denote the ribbon containing $j, j-1$ ($e_1, e_2$ not being necessarily different). Suppose*

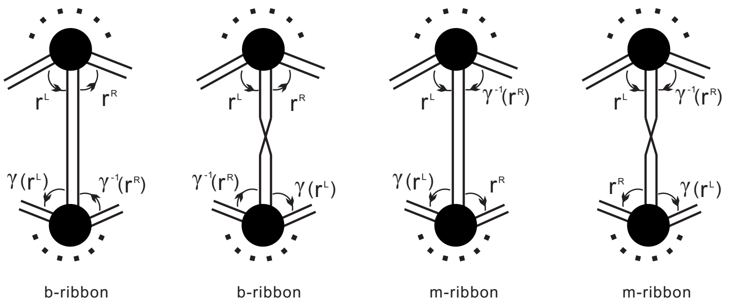


**Fig.** 3: $b$-ribbons and $m$-ribbons.

*that the ribbon* $r$ *contains* $\{r^L, \gamma(r^L), \gamma^{-1}(r^R), r^R\}$ *and* $r \neq e_1, r \neq e_2$. *Then*
(1) *the ribbon* $r^{i,j}$ *contains* $\{r^L, \gamma(r^L), \gamma^{-1}(r^R), r^R\}$,
(2) $e_1^{i,j}$ *contains sectors* $i+1, j$,
(3) $e_2^{i,j}$ *contains* $i, j-1$.

*Proof.* It is clear that any ribbon is determined by any two consecutive sectors, or by its origin and terminus. By construction, a reversal changes only two pairs of consecutive sectors on the boundary component, namely $i, i+1$ and $j-1, j$. As a result in $\tilde{\mathbb{G}}$, $r^{i,j}$ contains of the same sectors as $r$, $\{r^L, \gamma(r^L), \gamma^{-1}(r^R), r^R\}$. Furthermore $e_1^{i,j}$ is determined by the sectors $i+1, j$ and $e_2^{i,j}$ is determined by $i, j-1$. □

Let $\delta_r$ denote the *directional status* of $r$, indicating it being mono- or bi-directional.

*Proof of Lemma 2.* We consider the four sectors contained in $r$ as two pairs $\{r^L, \gamma(r^L)\}$ and $\{\gamma^{-1}(r^R), r^R\}$. In case of $r \neq e_1$ and $r \neq e_2$, Proposition 3 shows that $r^{i,j}$ consists of the same pairs, $\{r^L, \gamma(r^L)\}$ and $\{\gamma^{-1}(r^R), r^R\}$.

By the definition of $m$-ribbon and $b$-ribbon, see Fig. 3, $r$ changes its directional status if and only if exactly one pair of sectors changes their orientations.

**Claim 1:** if $r$ intersects the interval $[i, j]_\gamma$, then it changes $\delta_r$.

Without loss of generality, we assume that $r^L <_\gamma i <_\gamma r^R \leq_\gamma j$. Thus $r^L <_\gamma \gamma(r^L) \leq_\gamma i \leq_\gamma \gamma^{-1}(r^R) <_\gamma r^R \leq_\gamma j$. In view of eq. (4.2), only the sectors $i+1, \ldots, j-1$ change their orientations. This implies that the pair $\{r^L, \gamma(r^L)\}$ does not change orientations. For $\{\gamma^{-1}(r^R), r^R\}$, we have the following cases

1. $i <_\gamma \gamma^{-1}(r^R) <_\gamma r^R <_\gamma j$. By eq. (4.2), the sectors $\gamma^{-1}(r^R)$ and $r^R$ change orientation.
2. $i = \gamma^{-1}(r^R) <_\gamma i+1 = r^R <_\gamma j$. By Proposition 3, the $r$-pair $\{i, i+1\}$ becomes the $r^{i,j}$-pair $\{j, i+1\}$. By assumption, $i, j$ have different orientations. Thus, the pair $\{i, i+1\}$ of $r$ changes orientation.
3. $i <_\gamma \gamma^{-1}(r^R) = j-1 <_\gamma r^R = j$: this is analogous to the previous case.
4. $i = \gamma^{-1}(r^R) <_\gamma r^R = j$. Proposition 3 shows that the $r$-pair $\{i, j\}$ of $r$ becomes the $r^{i,j}$-pair $\{j, i\}$ of $r^{i,j}$. This implies that $\{i, j\}$ of $r$ changes orientation.

Since exactly one pair of sectors changes their orientations, $\delta_r$ changes.

It remains to show that

**Claim 2:** if $r$ does not intersect the interval $[i, j]_\gamma$, then it does not change its directional status. We distinguish the following cases

1. $r^L <_\gamma i <_\gamma j <_\gamma r^R$.
2. $r^L <_\gamma r^R \leq_\gamma i <_\gamma j$.
3. $i <_\gamma j \leq_\gamma r^L <_\gamma r^R$.
4. $i \leq_\gamma r^L <_\gamma r^R \leq_\gamma j$.

For cases (1)–(3), we check that both two pairs $\{r^L, \gamma(r^L)\}$ and $\{\gamma^{-1}(r^R), r^R\}$ do not change their orientations. In case of case (4), we verify that both pairs $\{r^L, \gamma(r^L)\}$ and $\{\gamma^{-1}(r^R), r^R\}$ change their orientations due to eq. (4.2). As a result $\delta_r$ does not change. □

## 3. The construction of $\tilde{T}$

We enhance Lemma 5 by giving an explicit construction of the component tree after the reversal. Let $\mathbb{G}$ be a unicellular fatgraph and $T$ be its component tree. Suppose that $i$ and $j$ are two sectors such that $i <_\gamma j$, and they are attached to two vertices $v_i$ and $v_j$ in $T$, respectively. Let $P^{i,j}$ denote the path joining $v_i$ and $v_j$ in $T$. Suppose that $P^{i,j}$ contains at least two $\mathbb{G}$-components.

Let $\tilde{\mathbb{G}}$ be the fatgraph obtained by the $i, j$-reversal and $\tilde{T}$ denote the component tree of $\tilde{\mathbb{G}}$. Lemma 5 gives us all $\tilde{\mathbb{G}}$-components, i.e., each $\mathbb{G}$-component not on the path $P^{i,j}$ is a $\tilde{\mathbb{G}}$-component and all components on the path $P^{i,j}$ form one $\tilde{\mathbb{G}}$-component $C_*$. To construct $\tilde{T}$, it remains to identify all $\tilde{\mathbb{G}}$-gaps and their adjacencies with $\tilde{\mathbb{G}}$-components.

An interval $[g_1, g_2]_\gamma$ *intersects* the interval $[i, j]_\gamma$ if $g_1 <_\gamma i <_\gamma g_2 \leq_\gamma j$ or $i \leq_\gamma g_1 <_\gamma j <_\gamma g_2$. Let $\tilde{g}$ denote the set of sectors from $[g_1, g_2]_\gamma$ obtained by the $i, j$-reversal. If $[g_1, g_2]_\gamma$ does not intersect $[i, j]_\gamma$, then by Lemma 1, $\tilde{\gamma}$ only reverses the part $i+1, \ldots, j-1$, and thus $\tilde{g}$ is still an interval, either $[g_1, g_2]_{\tilde{\gamma}}$ or $[g_2, g_1]_{\tilde{\gamma}}$. By abuse of notation, we use $[g_1, g_2]_\gamma$ to denote the interval $\tilde{g}$ obtained by the $i, j$-reversal.

Similar to Claim 1 and Claim 2 of Lemma 5, we have
**Claim:** a gap $[g_1, g_2]_\gamma$ is contained in $P^{i,j}$ if and only if it satisfies either

1. $g_1 \leq_\gamma i \leq_\gamma g_2 \leq_\gamma j$,
2. $i \leq_\gamma g_1 \leq_\gamma j \leq_\gamma g_2$,
3. $[g_1, g_2]_\gamma$ is the minimum common ancestor of $v_i$ and $v_j$ in $T$.

In the following we show how $\mathbb{G}$-gaps change by the reversal.

First consider a $\mathbb{G}$-gap $[g_1, g_2]_\gamma$ not contained in $P^{i,j}$. By the Claim, $[g_1, g_2]_\gamma$ does not intersect $[i, j]_\gamma$. Note that each child $C$ of $[g_1, g_2]_\gamma$ is either not contained in $P^{i,j}$ or the minimum common ancestor of $v_i$ and $v_j$ in $T$. By Claim 1 and Claim 2 of Lemma 5, the minimum and maximum sectors of the trace $I_C$ satisfy that $[\min I_C, \max I_C]_\gamma$ does not intersect $[i, j]_\gamma$. Since $\tilde{\gamma}$ only reverses within $i+1, \ldots, j-1$, by Lemma 1, all children of $[g_1, g_2]_\gamma$ are contained in $[g_1, g_2]_\gamma$ after the reversal, and therefore $[g_1, g_2]_\gamma$ is a $\tilde{\mathbb{G}}$-gap. Moreover, if $[g_1, g_2]_\gamma$ and a component not contained in $P^{i,j}$ are adjacent in $T$, so are they in $\tilde{T}$. If $[g_1, g_2]_\gamma$ is adjacent to a component contained in $P^{i,j}$, then $[g_1, g_2]_\gamma$ is adjacent to $C_*$ in $\tilde{T}$.

Now we consider a gap $[g_3, g_4]_\gamma$ contained in $P^{i,j}$. Let $v_0$ denote the minimum common ancestor of $v_i$ and $v_j$ in $T$. We distinguish the following cases

1. $[g_3, g_4]_\gamma \notin \{v_i, v_j, v_0\}$. By the Claim, we may assume that $g_3 <_\gamma i <_\gamma g_4 <_\gamma j$, and $g_3 = s^{(0)} <_\gamma \cdots <_\gamma s^{(k)} <_\gamma i <_\gamma s^{(k+1)} <_\gamma \cdots <_\gamma s^{(l)} = g_4$, where the children of $[g_3, g_4]_\gamma$ in $T$ are $C_h$ such that $\min I_{C_h} = s^{(h-1)}$ and $\max I_{C_h} = s^{(h)}$. Note that the component $C_{k+1}$ is the only child of $[g_3, g_4]_\gamma$ that is contained in $P^{i,j}$. Lemma 5 implies that the components $C_h$ form two new gaps after the reversal, i.e., $[g_3, s^{(k)}]_\gamma$ and $[s^{(k+1)}, g_4]_\gamma$. In $\tilde{T}$, both $[g_3, s^{(k)}]_\gamma$ and $[s^{(k+1)}, g_4]_\gamma$ are children of $C_*$, components $C_1, \ldots, C_k$ are children of $[g_3, s^{(k)}]_\gamma$ and components $C_{k+2}, \ldots, C_l$ are children of $[s^{(k+1)}, g_4]_\gamma$, see Fig. 4.
2. $[g_3, g_4]_\gamma$ is $v_i$, but not $v_0$. By definition, we have $g_3 \leq_\gamma i \leq_\gamma g_4 <_\gamma j$ and $g_3 = s^{(0)} <_\gamma \cdots <_\gamma s^{(k)} = i <_\gamma \cdots <_\gamma s^{(l)} = g_4$, where the children

of $[g_3, g_4]_\gamma$ in $T$ are the components $C_h$ such that $\min I_{C_h} = s^{(h-1)}$ and $\max I_{C_h} = s^{(h)}$. Then $[g_3, g_4]_\gamma$ is partitioned into two parts $[g_3, i]_\gamma$ and $[i, g_4]_\gamma$ by the $i, j$-reversal. We have the sub-cases

(a) $v_j$ is not a gap: in $\tilde{T}$, both $[g_3, i]_\gamma$ and $[i, g_4]_\gamma$ are children of $C_*$, components $C_1, \ldots, C_k$ are children of $[g_3, i]_\gamma$ and components $C_{k+1}, \ldots, C_l$ are children of $[i, g_4]_\gamma$, see Fig. 5.

(b) $v_j$ is a gap, which we denote by $[g_5, g_6]_\gamma$. Then the $i, j$-reversal, merges $[g_5, j]_\gamma$ with $[g_3, i]_\gamma$ and $[j, g_6]_\gamma$ with $[i, g_4]_\gamma$. Let $g^L_{i,j}$ denote $[g_3, g_5]_{\tilde{\gamma}}$ and $g^R_{i,j}$ denote $[g_4, g_6]_{\tilde{\gamma}}$. Therefore $g^L_{i,j}$ and $g^R_{i,j}$ become $\tilde{\mathbb{G}}$-gaps of $C_*$ in $\tilde{T}$. Moreover, components contained in $[g_3, i]_\gamma$ and $[g_5, j]_\gamma$ become children of $g^L_{i,j}$ and components contained in $[i, g_4]_\gamma$ and $[j, g_6]_\gamma$ become children of $g^R_{i,j}$, see Fig. 6.

3. $[g_3, g_4]_\gamma$ is $v_j$, but not $v_0$: the argument is as in the case of $v_j$ being a gap.
4. $[g_3, g_4]_\gamma$ is $v_0$. Let $C_0$ denote the parent of $v_0$ in $T$. We distinguish the sub-cases

(a) $v_0 \neq v_i$ and $v_0 \neq v_j$: by construction, we may assume that $g_3 = s^{(0)} <_\gamma \cdots <_\gamma s^{(k_1)} <_\gamma i <_\gamma s^{(k_1+1)} <_\gamma \cdots <_\gamma s^{(k_2)} <_\gamma j <_\gamma s^{(k_2+1)} <_\gamma \cdots <_\gamma s^{(l)} = g_4$, where the children of $[g_3, g_4]_\gamma$ in $T$ are the components $C_h$ such that $\min I_{C_h} = s^{(h-1)}$ and $\max I_{C_h} = s^{(h)}$. The components $C_{k_1+1}$ and $C_{k_2+1}$ are the only children of $[g_3, g_4]_\gamma$ that are contained in $P^{i,j}$. Lemma 5 shows that the components form three new gaps, i.e., $[g_3, s^{(k_1)}]_\gamma$ and $[s^{(k_1+1)}, s^{(k_2)}]_\gamma$ and $[s^{(k_2+1)}, g_4]_\gamma$. After the $i, j$-reversal, $[g_3, g_4]_\gamma$ is still a child of $C_0$, component $C_*$ becomes a child of $[g_3, g_4]_\gamma$ and the children of $[g_3, g_4]_\gamma$ are contained in $[g_3, s^{(k_1)}]_\gamma$ and $[s^{(k_2+1)}, g_4]_\gamma$ remain children of $[g_3, g_4]_\gamma$ in $\tilde{T}$. The interval $[s^{(k_1+1)}, s^{(k_2)}]_\gamma$ becomes a $\tilde{\mathbb{G}}$-gap of $C_*$ in $\tilde{T}$, while the children of $[g_3, g_4]_\gamma$ contained in $[s^{(k_1+1)}, s^{(k_2)}]_\gamma$ become children of $[s^{(k_1+1)}, s^{(k_2)}]_\gamma$ in $\tilde{T}$, see Fig. 7.

(b) $v_0 = v_i$, and $v_j$ is not a gap: by construction, we may assume that $g_3 = s^{(0)} <_\gamma \cdots <_\gamma s^{(k_1)} = i <_\gamma \cdots <_\gamma s^{(k_2)} <_\gamma j <_\gamma s^{(k_2+1)} <_\gamma \cdots <_\gamma s^{(l)} = g_4$, where the children of $[g_3, g_4]_\gamma$ in $T$ are the components $C_h$ such that $\min I_{C_h} = s^{(h-1)}$ and $\max I_{C_h} = s^{(h)}$. Component $C_{k_2+1}$ is the only child of $[g_3, g_4]_\gamma$ that is contained in $P^{i,j}$. We observe that components form the three new gaps, $[g_3, i]_\gamma$ and $[i, s^{(k_2)}]_\gamma$ and $[s^{(k_2+1)}, g_4]_\gamma$. After the $i, j$-reversal, $[g_3, g_4]_\gamma$ is remains to be a child of $C_0$, the component $C_*$ becomes a child of $[g_3, g_4]_\gamma$, and children of $[g_3, g_4]_\gamma$ contained in $[g_3, i]_\gamma$ and

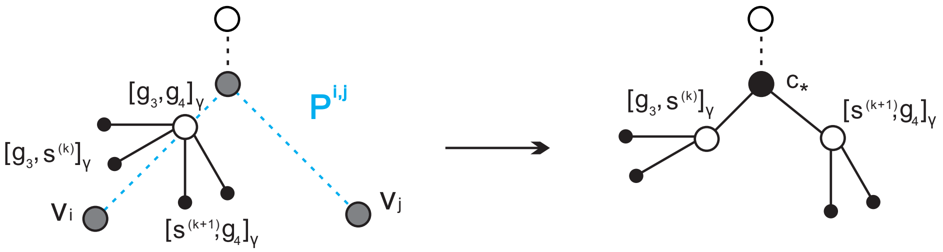


**Fig.** 4: Case (1).

$[s^{(k_2+1)}, g_4]_\gamma$ remain children of $[g_3, g_4]_\gamma$ in $\tilde{T}$. The interval $[i, s^{(k_2)}]_\gamma$ becomes a $\tilde{\mathbb{G}}$-gap of $C_*$ in $\tilde{T}$, while the children of $[g_3, g_4]_\gamma$ contained in $[i, s^{(k_2)}]_\gamma$ become children of $[i, s^{(k_2)}]_\gamma$ in $\tilde{T}$, see Fig. 8.

(c) $v_0 = v_i$ and $v_j$ is a gap, which we denote by $[g_5, g_6]_\gamma$. By construction, we may assume that $g_3 = s^{(0)} <_\gamma \cdots <_\gamma s^{(k_1)} = i <_\gamma \cdots <_\gamma s^{(k_2)} <_\gamma j <_\gamma s^{(k_2+1)} <_\gamma \cdots <_\gamma s^{(l)} = g_4$, where the children of $[g_3, g_4]_\gamma$ in $T$ are the $C_h$ such that $\min I_{C_h} = s^{(h-1)}$ and $\max I_{C_h} = s^{(h)}$. The component $C_{k_2+1}$ is the only child of $[g_3, g_4]_\gamma$ that is contained in $P^{i,j}$. Lemma 5 shows that the components form the three new gaps $[g_3, i]_\gamma$, $[i, s^{(k_2)}]_\gamma$ and $[s^{(k_2+1)}, g_4]_\gamma$. In difference to case 4(b), the $i, j$-reversal merges $[g_5, j]_\gamma$ with $[g_3, i]_\gamma$ as well as $[j, g_6]_\gamma$ with $[i, s^{(k_2)}]_\gamma$. Let $g^L_{i,j}$ denote $[g_3, g_5]_{\tilde{\gamma}}$ and $g^M_{i,j}$ denote $[s^{(k_2)}, g_6]_{\tilde{\gamma}}$. In $\tilde{T}$, the gap $[g_3, g_4]_\gamma$ remains to be a child of $C_0$, $C_*$ becomes a child of $[g_3, g_4]_\gamma$, and components contained in $g^L_{i,j}$ and $[s^{(k_2+1)}, g_4]_\gamma$ become children of $[g_3, g_4]_\gamma$. The interval $g^M_{i,j}$ becomes a $\tilde{\mathbb{G}}$-gap of $C_*$ in $\tilde{T}$, while components contained in $g^M_{i,j}$ become children of $g^M_{i,j}$ in $\tilde{T}$, see Fig. 9.

(d) $v_0 = v_j$: this case is analogous to the cases 4(b) and 4(c).

Both: Proposition 4 and Proposition 5 follow directly from our construction of $\tilde{T}$. For example, if two $\mathbb{G}$-components are adjacent to a gap contained in $P^{i,j}$, they are either adjacent to each other or both of them adjacent to $C_*$ in $\tilde{\mathbb{G}}$. Therefore they are contained in the same $\tilde{\mathbb{G}}$-block.

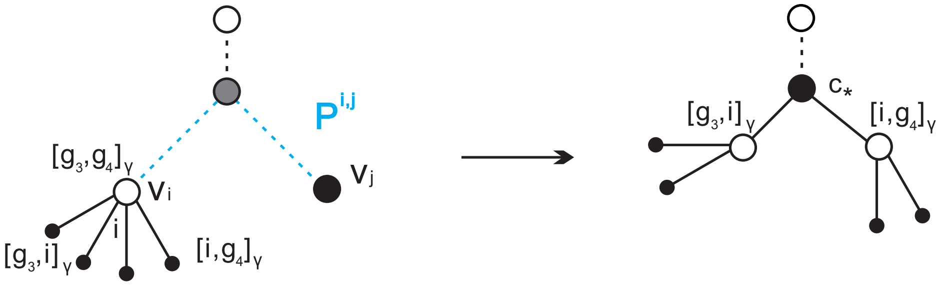


**Fig.** 5: Case (2a).

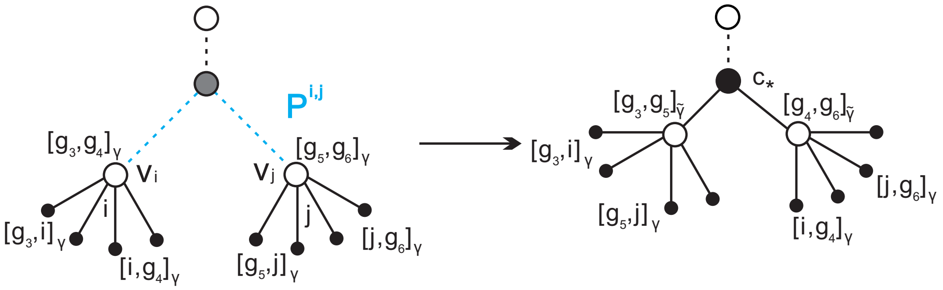


**Fig.** 6: Case (2b).

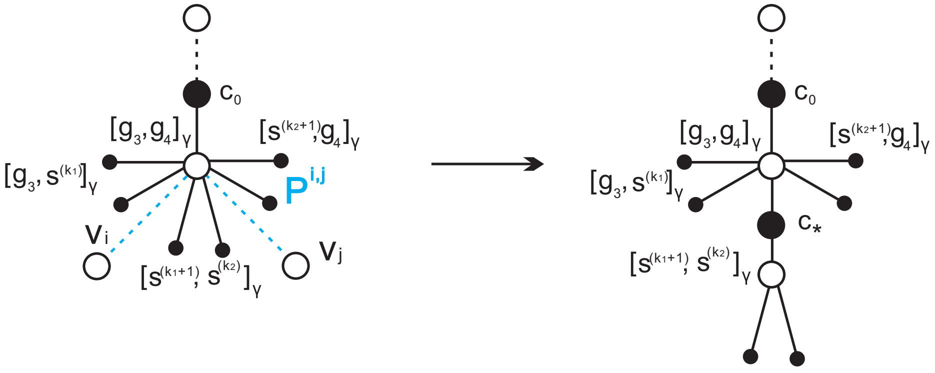


**Fig.** 7: Case (3a).

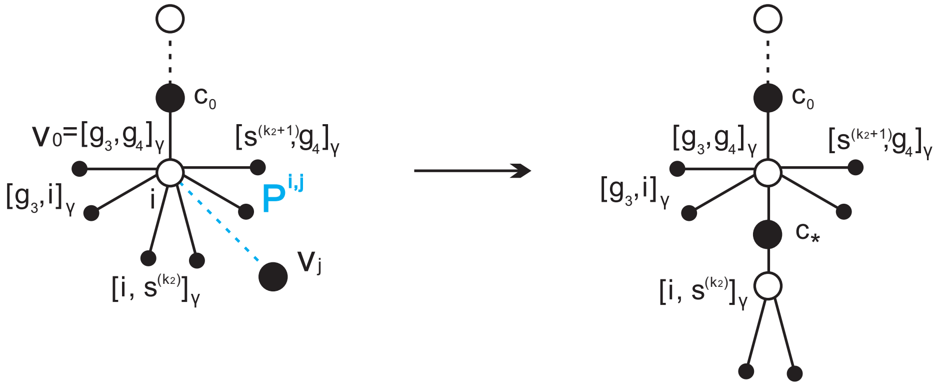


**Fig.** 8: Case (3b).

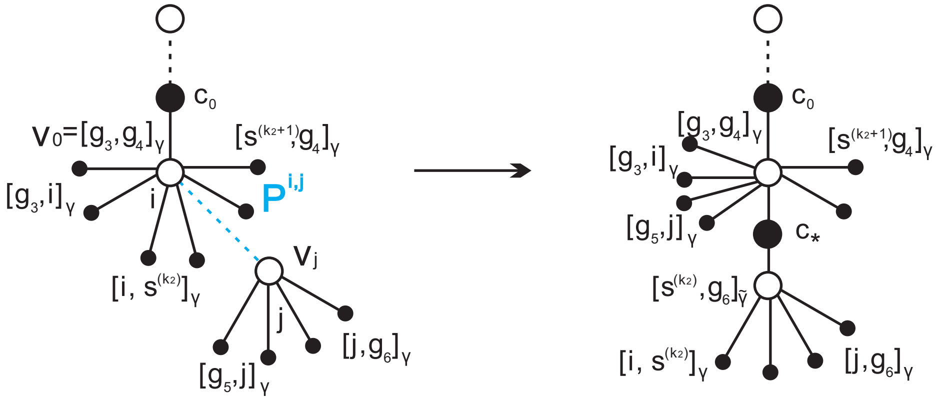


**Fig.** 9: Case (3c).
